# Supplementary material for: Elastic-dLLM: Position Preserving Context Compression and Augmentation of Diffusion LLMs
Source: arXiv:2605.18165 source file (2026-05-18)
Supplement: Supplementary file 1 [file appendix.tex]

\section{Additional Analysis}
\label{app:additional_analysis}

The appendix is organized around the three design signals used by Elastic-dLLM. First, future \texttt{[MASK]} tokens are active in attention but exhibit repeated and structured patterns, which motivates compressing them. Second, the final RoPE region carries a terminal signal for EOS prediction, which motivates preserving the terminal block in full-sequence dLLMs and adding a protected terminal anchor in block dLLMs. Third, RoPE coordinates affect generation behavior directly, which motivates preserving original positions rather than re-indexing retained tokens after compression.

\subsection{Additional \texttt{[MASK]} Attention Maps}
\label{app:attention_maps}

The attention analysis in Section~\ref{sec:mask_token_cost} uses one representative attention map. Figures~\ref{fig:app_attn_step16}--\ref{fig:app_attn_step480} show additional maps collected from different denoising stages and layers on a coding prompt. These plots are useful because they separate two facts that are easy to conflate. On the one hand, \texttt{[MASK]} tokens are not padding: they participate in attention and therefore contribute real computation. On the other hand, the patterns inside the masked region are highly regular, which means the future masked context contains redundant computation that can be represented sparsely.

\subsection{Terminal Signal Across Prompt Types}
\label{app:eos_signal}

Section~\ref{sec:eos_observation} argues that the final position in the planned generation context acts as a terminal signal. The figures below show that this behavior appears across different prompt families. The red trajectory in each plot tracks the position with the highest EOS probability during denoising. Although the exact trajectory depends on the task, the model often assigns strong EOS probability near the terminal region before the final answer is fully settled.

\begin{figure}[t]
    \centering
    \includegraphics[width=0.82\linewidth]{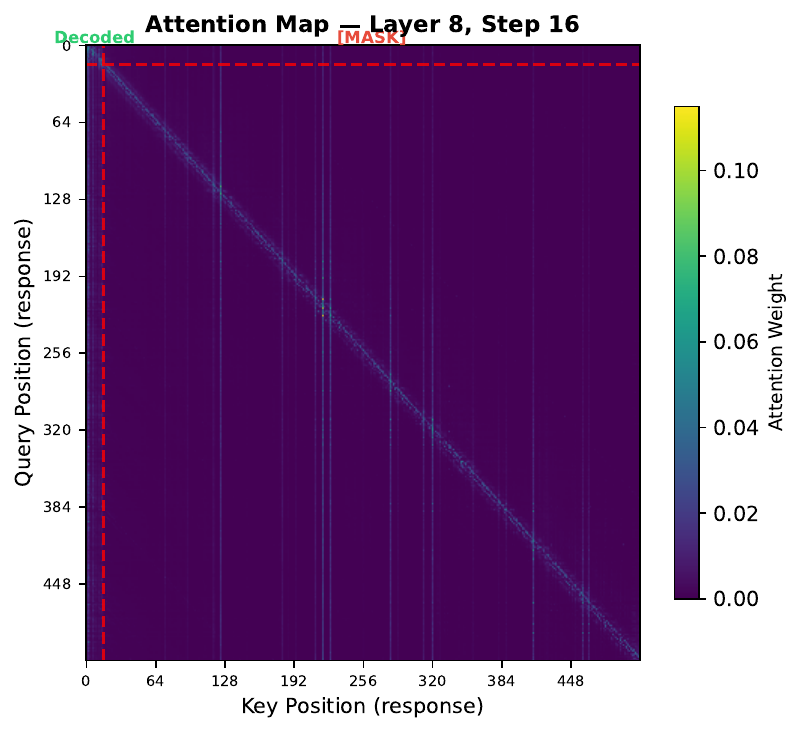}
    \caption{\textbf{Additional attention map at step 16, layer 8.} Even early in denoising, the masked region forms a structured attention pattern rather than behaving like inactive padding.}
    \label{fig:app_attn_step16}
\end{figure}

\begin{figure}[t]
    \centering
    \includegraphics[width=0.82\linewidth]{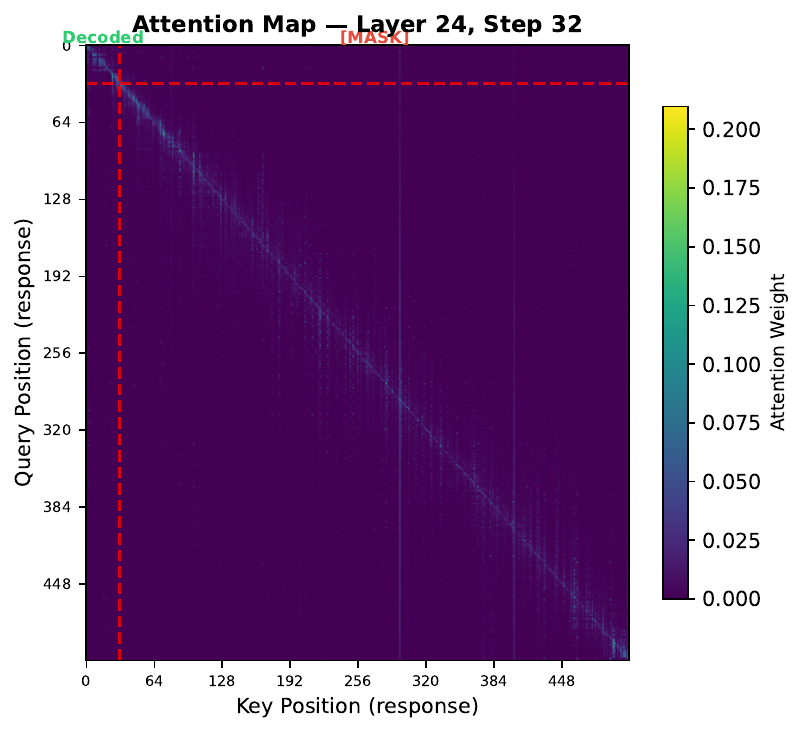}
    \caption{\textbf{Additional attention map at step 32, layer 24.} The masked positions continue to interact in a regular way, supporting sparse representation of future masked blocks.}
    \label{fig:app_attn_step32}
\end{figure}

\begin{figure}[t]
    \centering
    \includegraphics[width=0.82\linewidth]{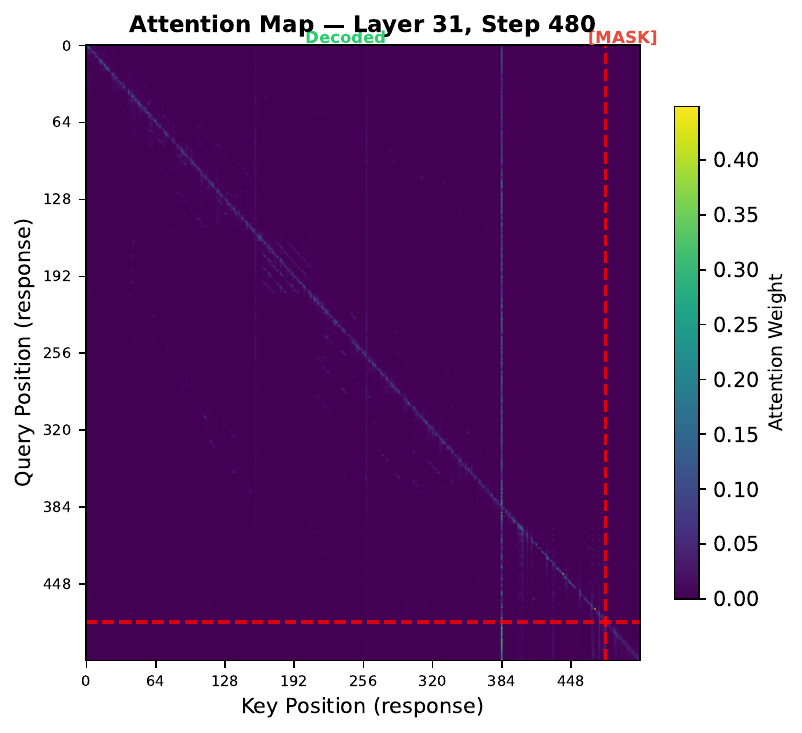}
    \caption{\textbf{Additional attention map at step 480, layer 31.} Near the end of denoising, masked-token computation remains structured, which is consistent with the redundancy exploited by Elastic-dLLM.}
    \label{fig:app_attn_step480}
\end{figure}
\begin{figure}[t]
    \centering
    \includegraphics[width=0.78\linewidth]{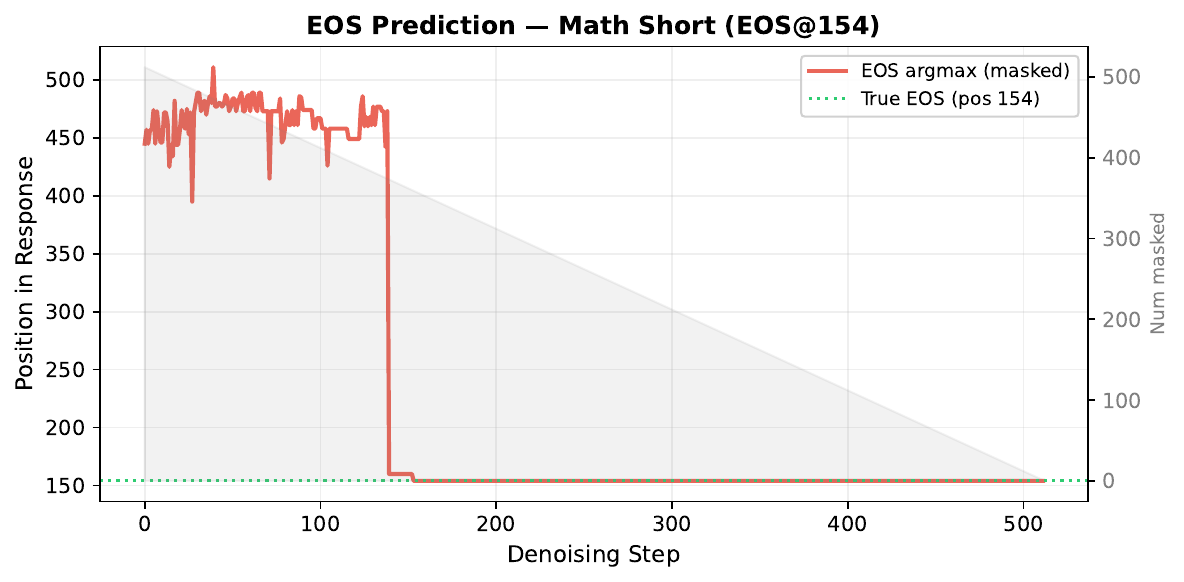}
    \caption{\textbf{EOS argmax on a short math prompt.} The EOS-preferred position is tied to the planned terminal region during denoising.}
    \label{fig:app_eos_math_short}
\end{figure}

\begin{figure}[t]
    \centering
    \includegraphics[width=0.78\linewidth]{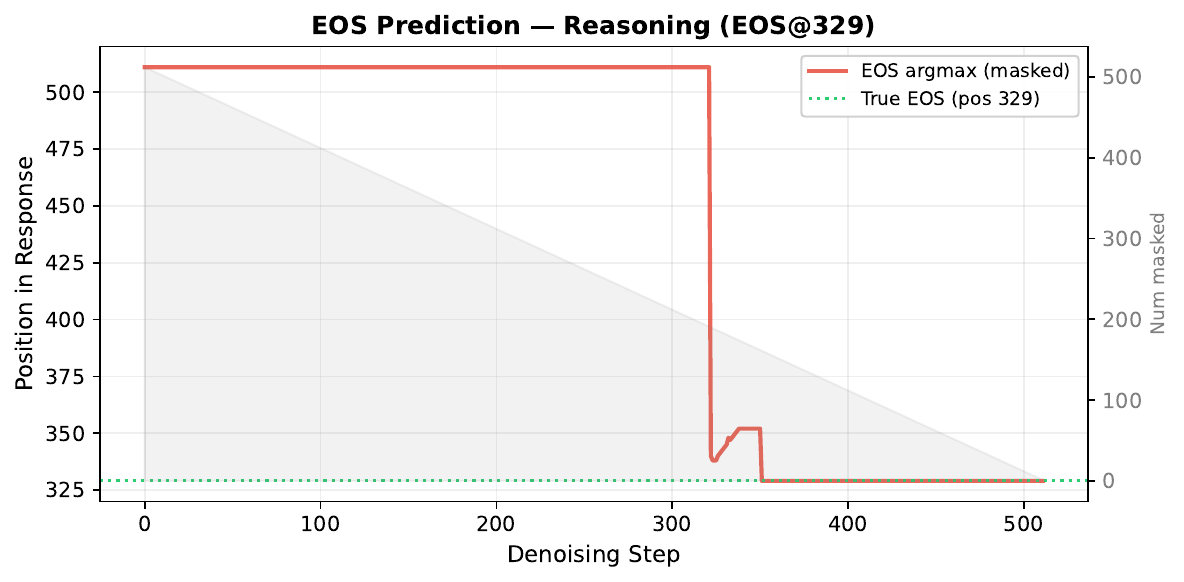}
    \caption{\textbf{EOS argmax on a reasoning prompt.} The terminal-region pattern also appears in a reasoning setting, suggesting that the final coordinate provides a general boundary cue.}
    \label{fig:app_eos_reasoning}
\end{figure}

\begin{figure}[t]
    \centering
    \includegraphics[width=0.78\linewidth]{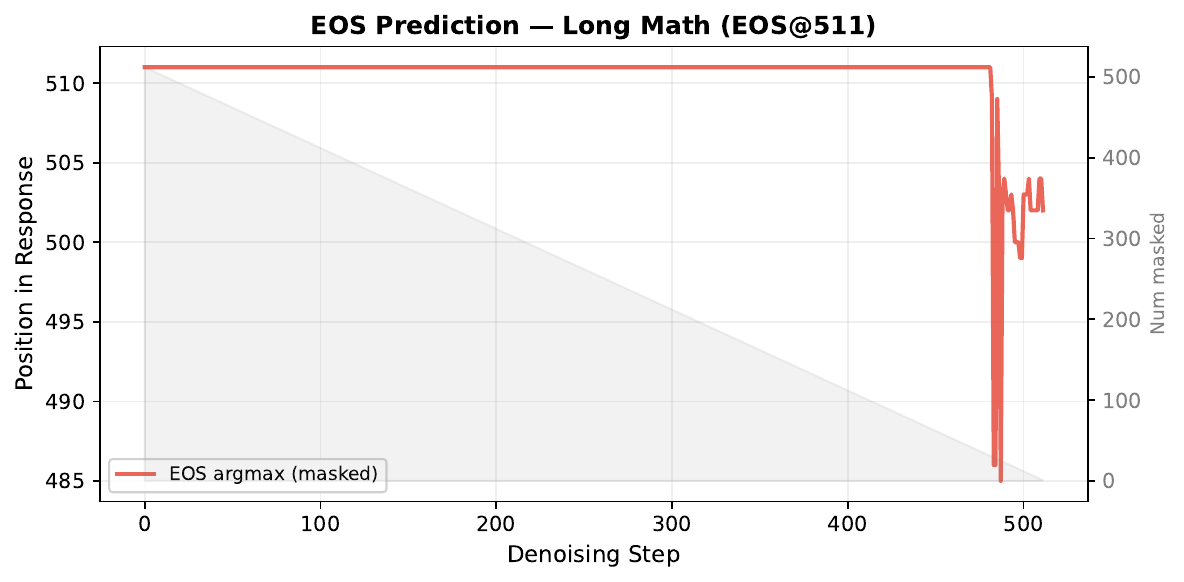}
    \caption{\textbf{EOS argmax on a long math prompt.} For longer generations, the planned terminal position remains informative before decoding converges to the final emitted EOS token.}
    \label{fig:app_eos_long_math}
\end{figure}

\begin{figure}[t]
    \centering
    \includegraphics[width=0.78\linewidth]{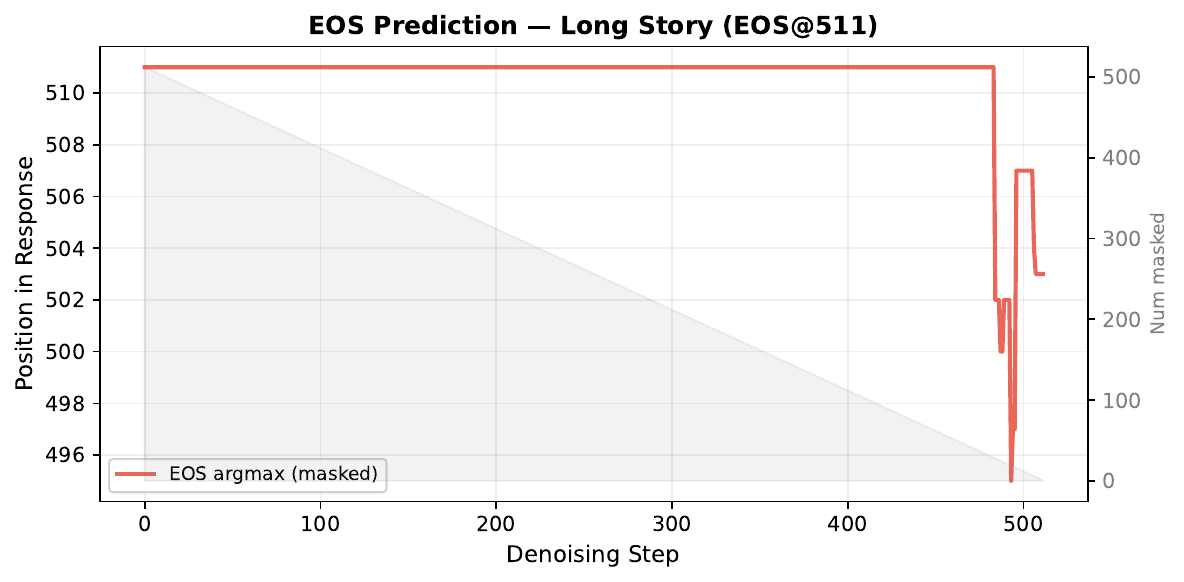}
    \caption{\textbf{EOS argmax on a long story prompt.} Open-ended generation still shows a terminal-region signal, which motivates keeping the end of the planned context visible.}
    \label{fig:app_eos_long_story}
\end{figure}

\begin{figure}[t]
    \centering
    \includegraphics[width=0.78\linewidth]{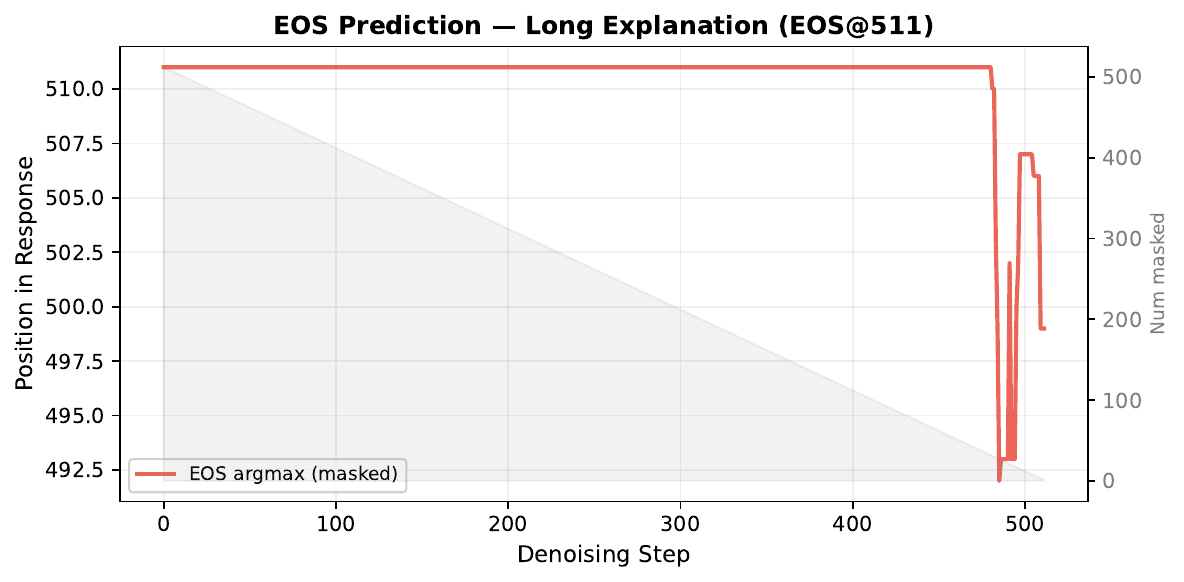}
    \caption{\textbf{EOS argmax on a long explanation prompt.} The trajectory indicates that EOS prediction depends on the planned generation boundary rather than only local semantics.}
    \label{fig:app_eos_long_explanation}
\end{figure}

\begin{figure}[t]
    \centering
    \includegraphics[width=0.78\linewidth]{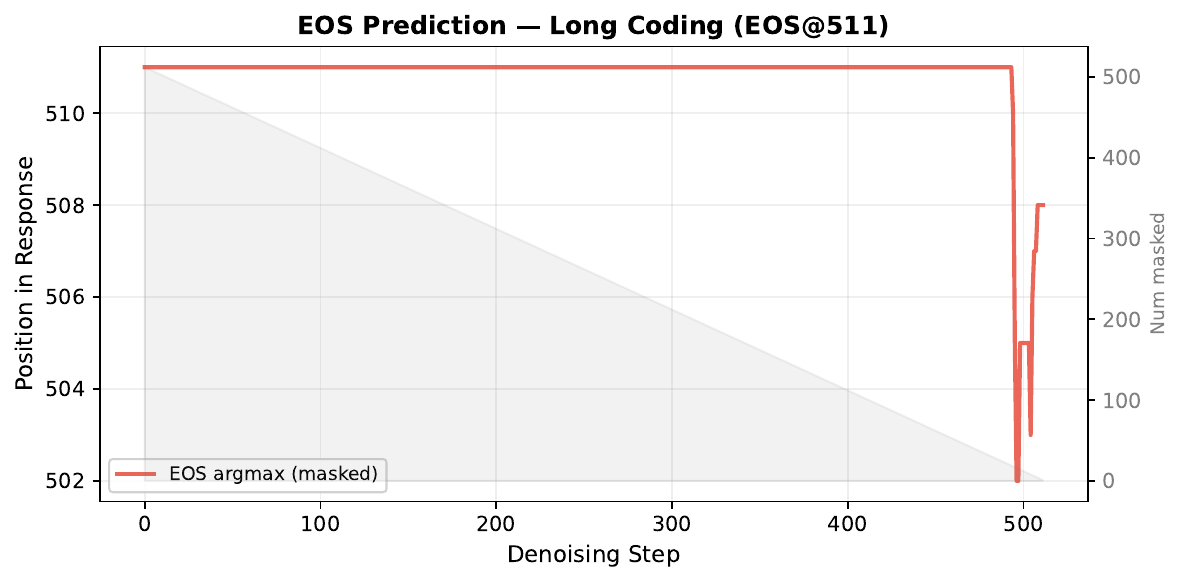}
    \caption{\textbf{EOS argmax on a long coding prompt.} The coding example further supports the terminal-anchor design used for block dLLMs.}
    \label{fig:app_eos_long_coding}
\end{figure}

\subsection{Additional Positional and Representation Visualizations}
\label{app:positional_representation}

The RoPE ablation in Table~\ref{tab:rope_ablation} shows that compacting the token layout is not enough: retained tokens must preserve their original RoPE coordinates. Figures~\ref{fig:app_positional_obs1} and \ref{fig:app_positional_obs2} provide qualitative examples behind this result. When a generated region receives a different RoPE coordinate, the generated content shifts toward the content associated with that coordinate. This suggests that position acts as a generation prior in dLLMs.

\begin{figure}[t]
    \centering
    \includegraphics[width=0.95\linewidth]{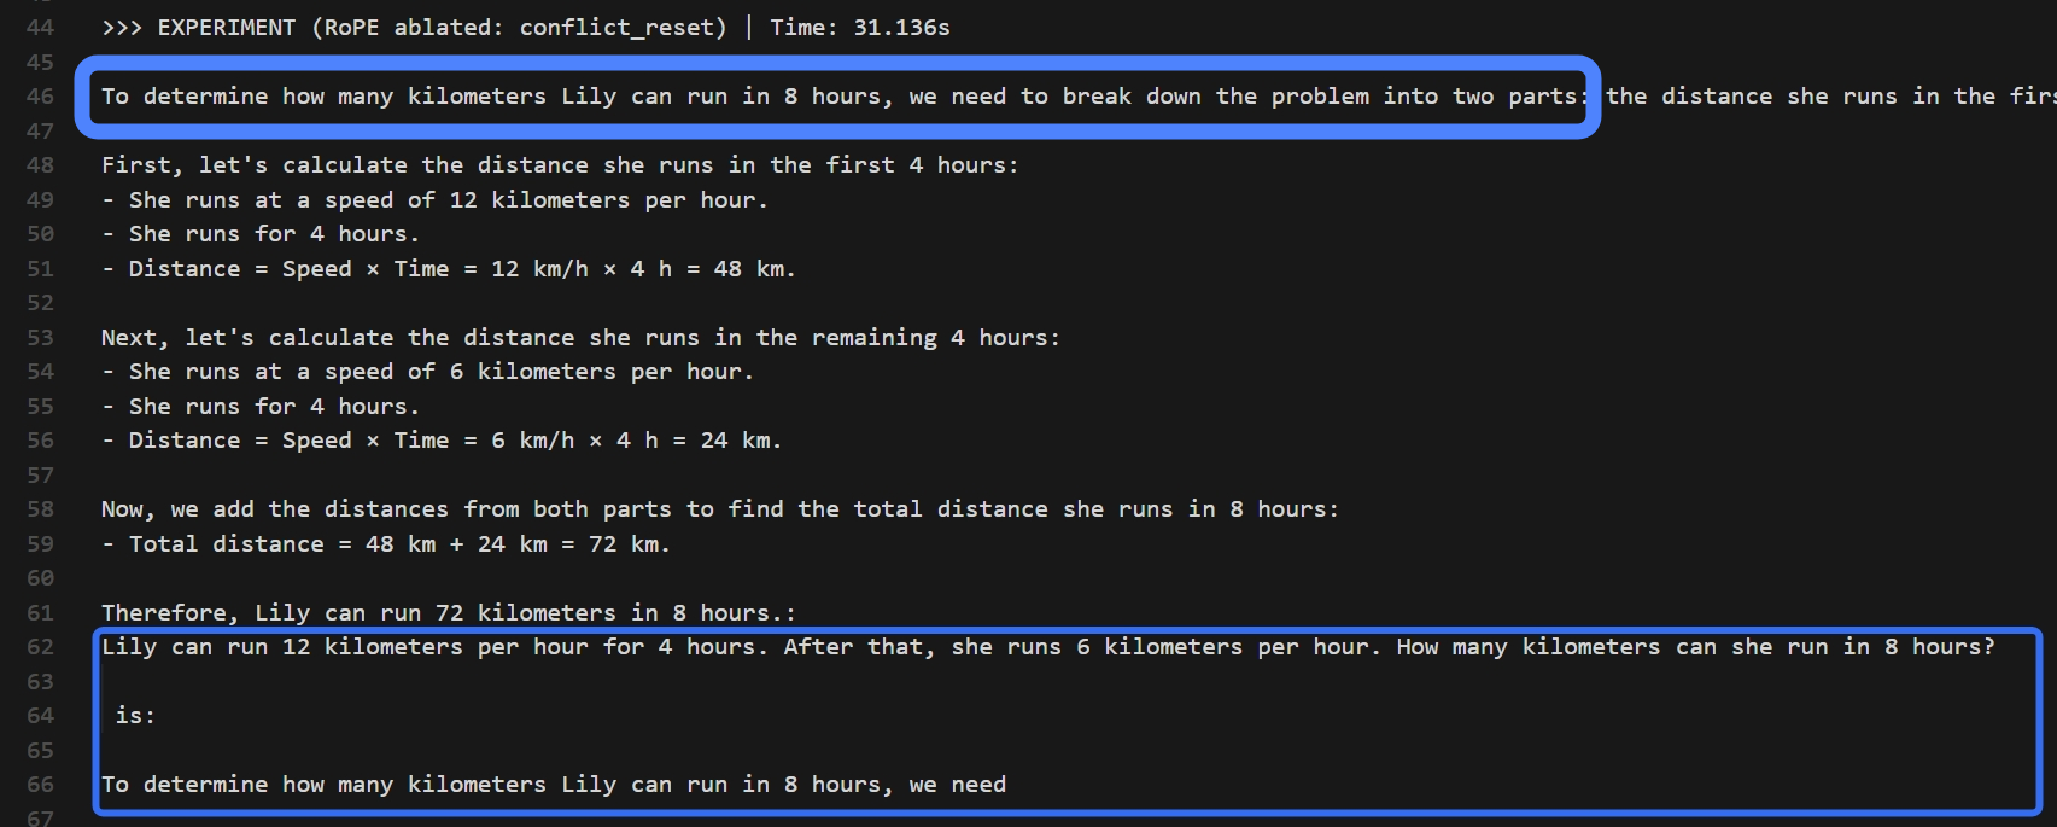}
    \caption{\textbf{Additional positional observation I.} RoPE coordinate assignment changes the generation prior, indicating that retained tokens should not be re-indexed after compression.}
    \label{fig:app_positional_obs1}
\end{figure}

\begin{figure}[t]
    \centering
    \includegraphics[width=0.95\linewidth]{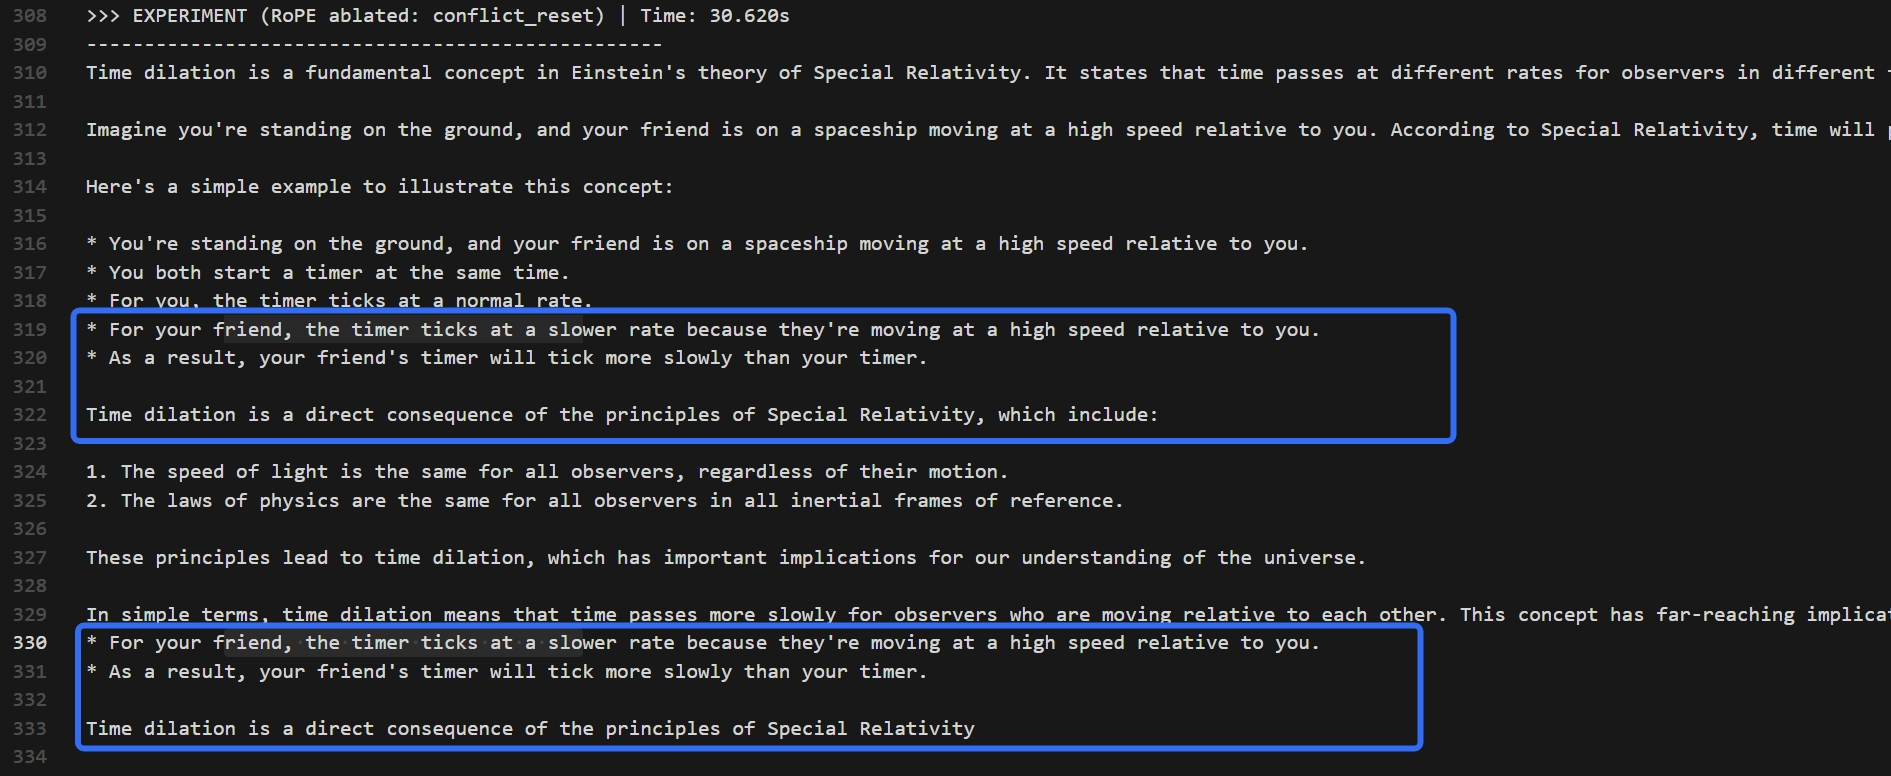}
    \caption{\textbf{Additional positional observation II.} A second qualitative example further supports preserving original RoPE coordinates in the compressed layout.}
    \label{fig:app_positional_obs2}
\end{figure}

\subsection{Reproducibility Details}
\label{app:impl}

Elastic-dLLM is training-free. For full-sequence dLLMs, we use the same model weights and decoding hyperparameters as the corresponding baseline. At each denoising stage, the compact layout keeps the decoded history, the current denoising block, and the terminal block dense. Middle future \texttt{[MASK]} blocks are compressed by uniformly retaining $r=8$ tokens from each block. This sampling is deterministic in our implementation once the block partition is fixed, and it does not require learning a token scorer.

All retained positions keep their original RoPE coordinates. This detail is essential: the compressed input is shorter in token count, but it still spans the same planned generation coordinate system. A compact-coordinate variant would assign retained tokens to consecutive indices inside the shortened input. Table~\ref{tab:rope_ablation} shows that this alternative performs substantially worse, which matches the positional observations above.

For block dLLMs, the only architectural change is one additional protected \texttt{[MASK]} token. This token is appended to the active input for attention computation, assigned to the final planned RoPE coordinate, and discarded before committing output tokens. It is not decoded into text and is rebuilt at each block step. Because the method adds only one token, its computational overhead is negligible relative to the current block.

For the standard benchmarks, accuracy is reported after rounding to two decimal places from integer counts. The evaluation set sizes are 500 for MATH500, 1,319 for GSM8K, 2,305 for ASDiv, 256 for Countdown, 164 for HumanEval, and 541 for IFEval. Countdown and MATH500 ablations in Table~\ref{tab:ablation} therefore use percentages aligned with 256 and 500 samples respectively.

\clearpage
